# Supplementary material for: Conservative Predictions on Noisy Financial Data
Source: arXiv:2310.11815 source file (2023-10-18)
Supplement: Supplementary file 1 [file appendix.tex]

\onecolumn
\section{Baseline models results on Synthetic Data}
\begin{table}[h]
\begin{subtable}[h]{0.40\textwidth}
    \centering
    % [inline block 0: 56 envs, 50831 chars -> data_tex | \begin{tabular}{|l|l|l|l|l|l|l|l|}     \hline...]

    \caption{Experiment 2 - Train-Test Support and Accuracy for base and Cascaded Models}
\end{table}
\clearpage
\section{Confusion Matrices for Experiment 1}
\begin{figure}[!ht]
  \centering
  \begin{subfigure}[b]{0.45\textwidth}
   \includegraphics[width=\textwidth]{confusion matrices/same set/ddt_[0.075,0.05]_base.png}
    \caption{Base DDT}
  \end{subfigure}
  \hfill
  \begin{subfigure}[b]{0.45\textwidth}
    \includegraphics[width=\textwidth]{confusion matrices/same set/ddt_[0.075,0.05]_cascaded.png}
    \caption{Cascaded DDT}
  \end{subfigure}
   \caption{ Confusion Matrices for DDT in Experiment 1 on
synthetic data with noise level [0.075,0.05]}
\end{figure}
\begin{figure}[!ht]
  \centering
  \begin{subfigure}[b]{0.45\textwidth}
   \includegraphics[width=\textwidth]{confusion matrices/same set/mlp_[0.075,0.05]_base.png}
    \caption{Base MLP}
  \end{subfigure}
  \hfill
  \begin{subfigure}[b]{0.45\textwidth}
    \includegraphics[width=\textwidth]{confusion matrices/same set/mlp_[0.075,0.05]_cascaded.png}
    \caption{Cascaded MLP}
  \end{subfigure}
   \caption{ Confusion Matrices for MLP in Experiment 1 on
synthetic data with noise level [0.075,0.05]}
\end{figure}
\begin{figure}[!ht]
  \centering
  \begin{subfigure}[b]{0.45\textwidth}
   \includegraphics[width=\textwidth]{confusion matrices/same set/ddt_market_base.png}
    \caption{Base DDT}
  \end{subfigure}
  \hfill
  \begin{subfigure}[b]{0.45\textwidth}
    \includegraphics[width=\textwidth]{confusion matrices/same set/ddt_market_cascaded.png}
    \caption{Cascaded DDT}
  \end{subfigure}
   \caption{ Confusion Matrices for DDT in Experiment 1 on
market data}
\end{figure}
\begin{figure}[!ht]
  \centering
  \begin{subfigure}[b]{0.45\textwidth}
   \includegraphics[width=\textwidth]{confusion matrices/same set/mlp_market_base.png}
    \caption{Base MLP}
  \end{subfigure}
  \hfill
  \begin{subfigure}[b]{0.45\textwidth}
    \includegraphics[width=\textwidth]{confusion matrices/same set/mlp_market_cascaded.png}
    \caption{Cascaded MLP}
  \end{subfigure}
   \caption{ Confusion Matrices for MLP in Experiment 1 on
market data}
\end{figure}
\clearpage
\section{Some results for Experiment 4}
\subsection{Synthetic Data (Noise Level: [0.075,0.05])}
\begin{figure}[!ht]
  \centering
  \begin{subfigure}[b]{0.45\textwidth}
   \includegraphics[width=\textwidth]{baseline scatter plots/regression_[0.075,0.05].png}
    \caption{Regression RMSE - Train vs Test}
  \end{subfigure}
  \hfill
  \begin{subfigure}[b]{0.45\textwidth}
    \includegraphics[width=\textwidth]{baseline scatter plots/classification_[0.075,0.05].png}
    \caption{Classification Accuracy - Train vs Test}
  \end{subfigure}
   \caption{ Scatter Plots for Baseline Models on
synthetic data (Train Era vs Test Era)}
\end{figure}
\begin{figure}[!ht]
  \centering
  \begin{subfigure}[b]{0.45\textwidth}
   \includegraphics[width=\textwidth]{scatter plots/ddt_[0.075,0.05]_accs.png}
    \caption{DDT Accuracy - Train vs Test}
  \end{subfigure}
  \hfill
  \begin{subfigure}[b]{0.45\textwidth}
    \includegraphics[width=\textwidth]{scatter plots/ddt_[0.075,0.05]_support.png}
    \caption{DDT Support - Train vs Test}
  \end{subfigure}
   \caption{ Scatter Plots for DDT on
synthetic data (Train Era vs Test Era)}
\end{figure}
\begin{figure}[!ht]
  \centering
  \begin{subfigure}[b]{0.45\textwidth}
   \includegraphics[width=\textwidth]{scatter plots/mlp_[0.075,0.05]_accs.png}
    \caption{MLP Accuracy - Train vs Test}
  \end{subfigure}
  \hfill
  \begin{subfigure}[b]{0.45\textwidth}
    \includegraphics[width=\textwidth]{scatter plots/mlp_[0.075,0.05]_support.png}
    \caption{MLP Support - Train vs Test}
  \end{subfigure}
   \caption{ Scatter Plots for MLP on
synthetic data (Train Era vs Test Era)}
\end{figure}
\clearpage
\subsection{Market Data}
\begin{figure}[!ht]
  \centering
  \begin{subfigure}[b]{0.45\textwidth}
   \includegraphics[width=\textwidth]{baseline scatter plots/regression_market.png}
    \caption{Regression RMSE - Train vs Test}
  \end{subfigure}
  \hfill
  \begin{subfigure}[b]{0.45\textwidth}
    \includegraphics[width=\textwidth]{baseline scatter plots/classification_market.png}
    \caption{Classification Accuracy - Train vs Test}
  \end{subfigure}
   \caption{ Scatter Plots for Baseline Models on
market data (Train Era vs Test Era)}
\end{figure}
\begin{figure}[!ht]
  \centering
  \begin{subfigure}[b]{0.45\textwidth}
   \includegraphics[width=\textwidth]{scatter plots/ddt_market_accs.png}
    \caption{DDT Accuracy - Train vs Test}
  \end{subfigure}
  \hfill
  \begin{subfigure}[b]{0.45\textwidth}
    \includegraphics[width=\textwidth]{scatter plots/ddt_market_support.png}
    \caption{DDT Support - Train vs Test}
  \end{subfigure}
   \caption{ Scatter Plots for DDT on
market data (Train Era vs Test Era)}
\end{figure}
\begin{figure}[!ht]
  \centering
  \begin{subfigure}[b]{0.45\textwidth}
   \includegraphics[width=\textwidth]{scatter plots/mlp_market_accs.png}
    \caption{MLP Accuracy - Train vs Test}
  \end{subfigure}
  \hfill
  \begin{subfigure}[b]{0.45\textwidth}
    \includegraphics[width=\textwidth]{scatter plots/mlp_market_support.png}
    \caption{MLP Support - Train vs Test}
  \end{subfigure}
   \caption{ Scatter Plots for MLP on
market data (Train Era vs Test Era)}
\end{figure}
